# Supplementary material for: DisPositioNet: Disentangled Pose and Identity in Semantic Image Manipulation
Source: arXiv:2211.05499 source file (2022-11-10)
Supplement: Supplementary file 1 [file 6_supplement.tex]

\section{Graphical Model}
A graphical model of our method compared to SIMSG \cite{dhamo2020semantic} can be seen in \cref{fig:graphical_model}.
\begin{figure}[htb]
    \centering
    \includegraphics[width=0.9\linewidth]{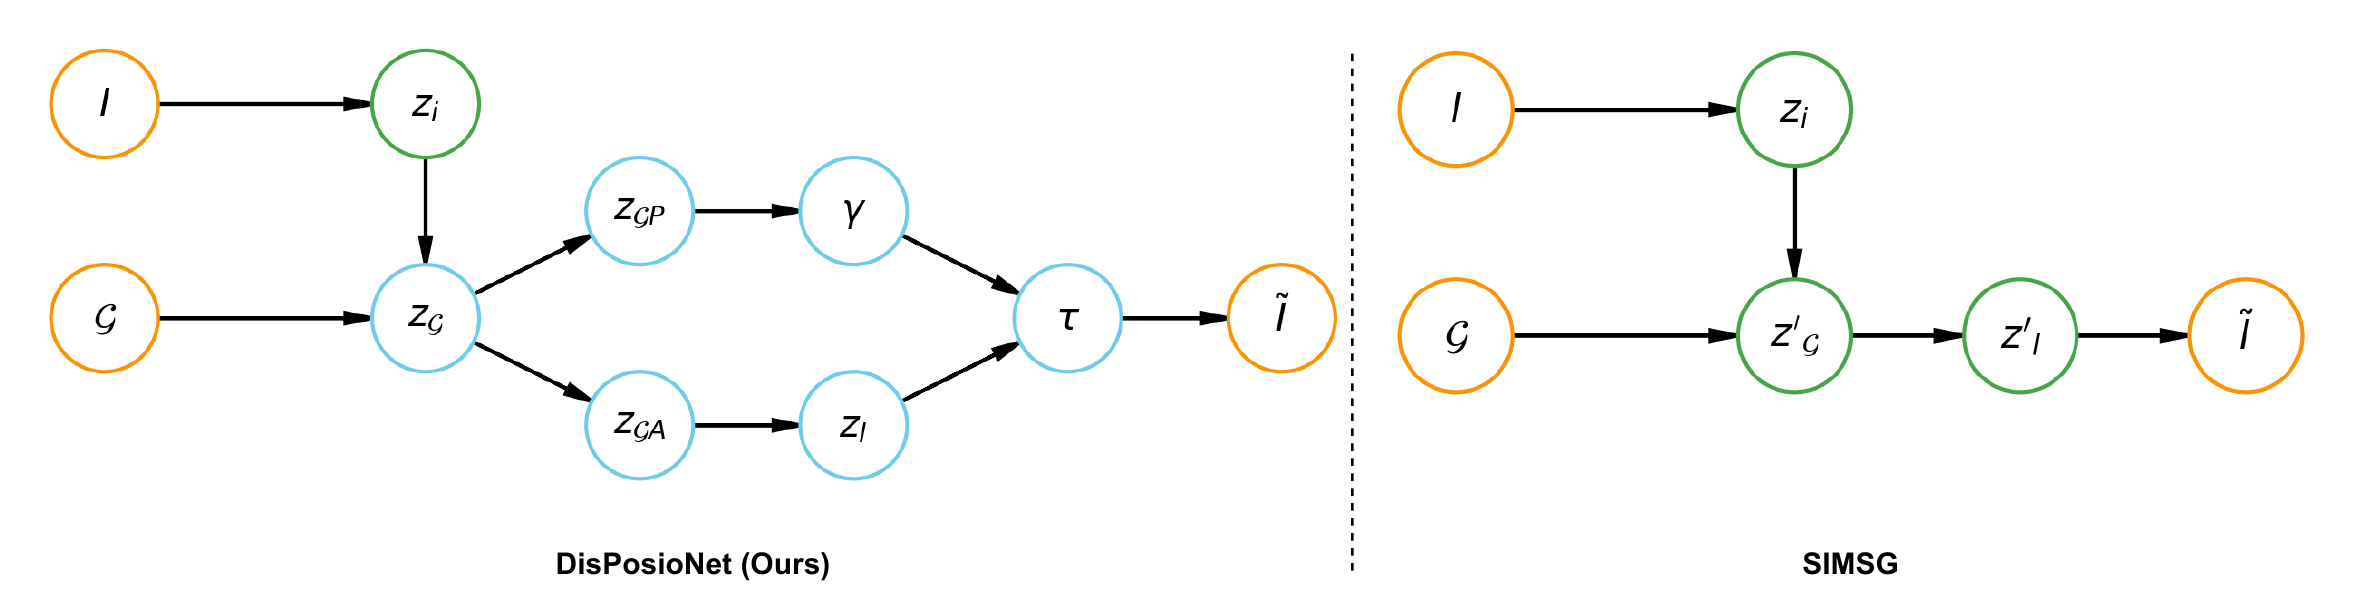}
    \caption{\textbf{A graphical model of our approach compared to SIMSG \cite{dhamo2020semantic}.} The inputs to both models are image $I$ and scene graph $\mathcal{G}$. The differences between the two methods are shown by the blue color. While SIMSG reconstructs the image directly from the latent embedding $z_l$, \methodName{} disentangles both the graph representation and the latent embeddings.}
    \label{fig:graphical_model}
\end{figure}

\section{Results on COCO \cite{lin2014microsoft}}
The qualitative results on the COCO \cite{lin2014microsoft} dataset are presented in \cref{fig:qual_res_coco}. As it can be seen, our model predicts the target bounding box for repositioning the object more effectively due to the disentanglement of pose and appearance. The modifications by our model have less artefacts and look more realistic compared to the baseline model. %quantitative and  \cref{tab:coco} 

\begin{figure}[!htb]
    \centering
    \includegraphics[height=0.9\textheight]{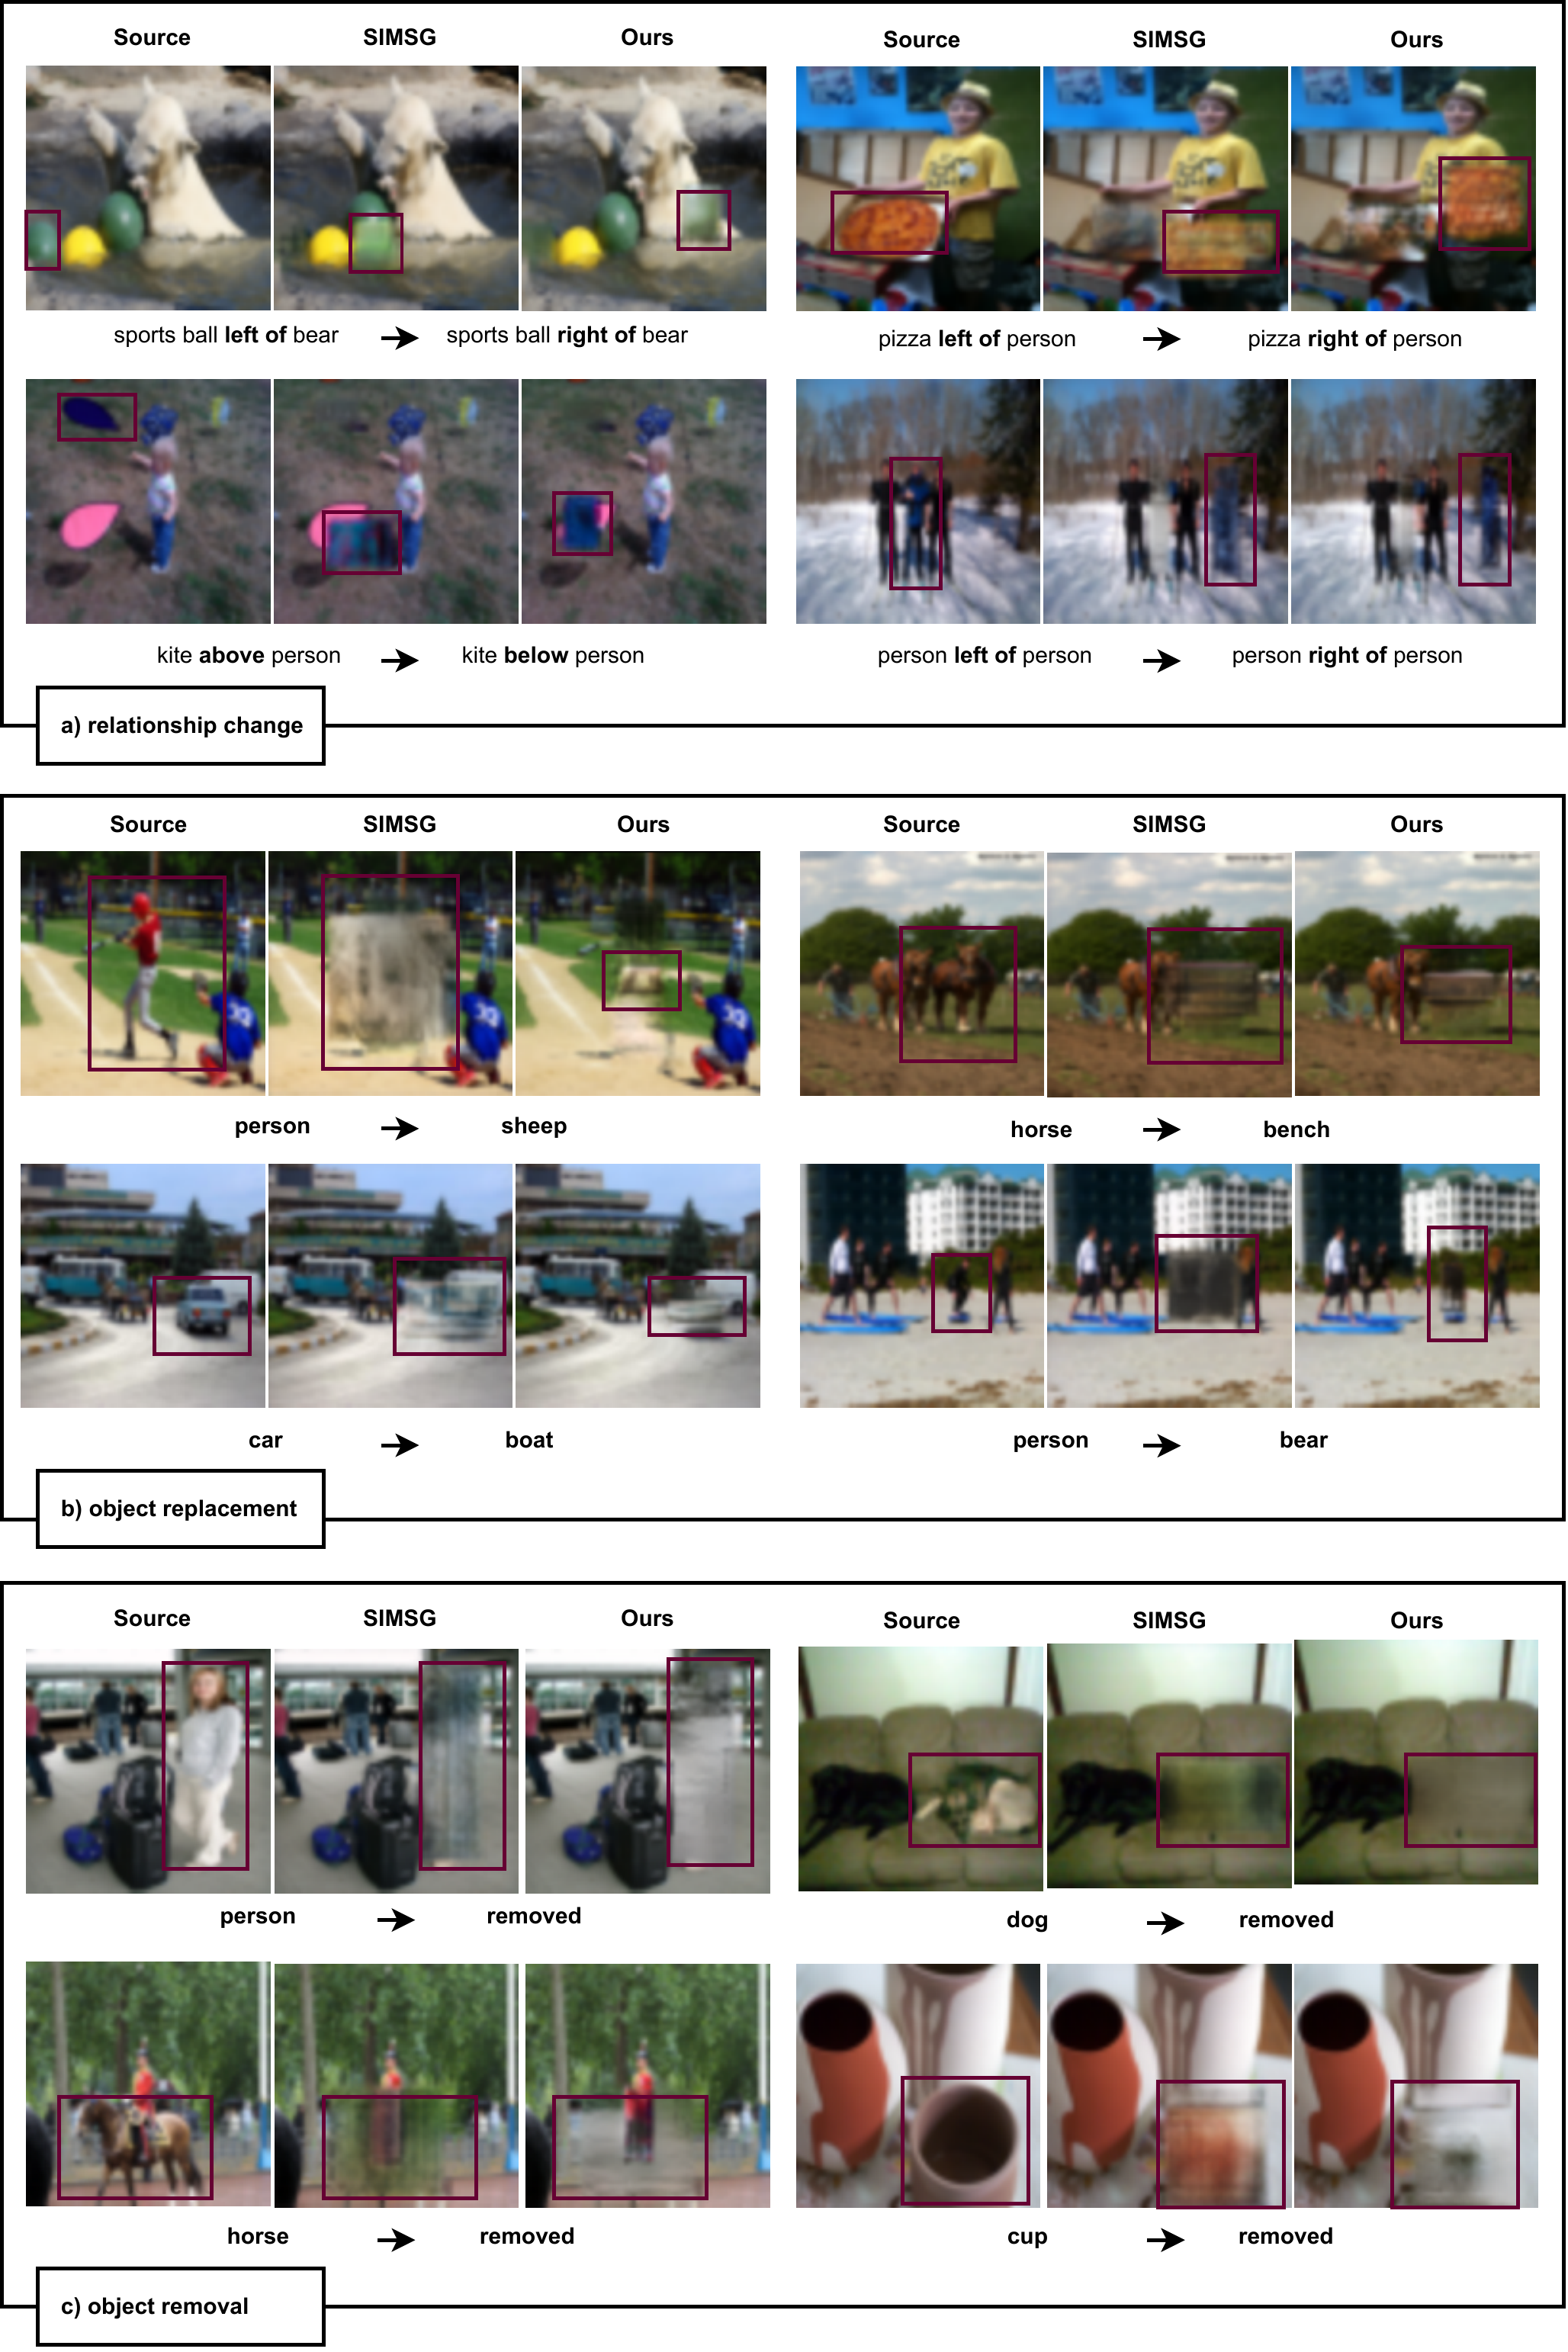}
    \caption{Qualitative results for image manipulation on COCO}
    \label{fig:qual_res_coco}
\end{figure}

\section{Additional Qualitative Results on VG \cite{krishna2017visual}}
More qualitative results compared to \cite{dhamo2020semantic} are provided in \cref{fig:qual_res}. Similar to the results on the COCO dataset, our model modifies the objects more realistically on the VG dataset.
\begin{figure}[!htb]
    \centering
    \includegraphics[height=0.9\textheight]{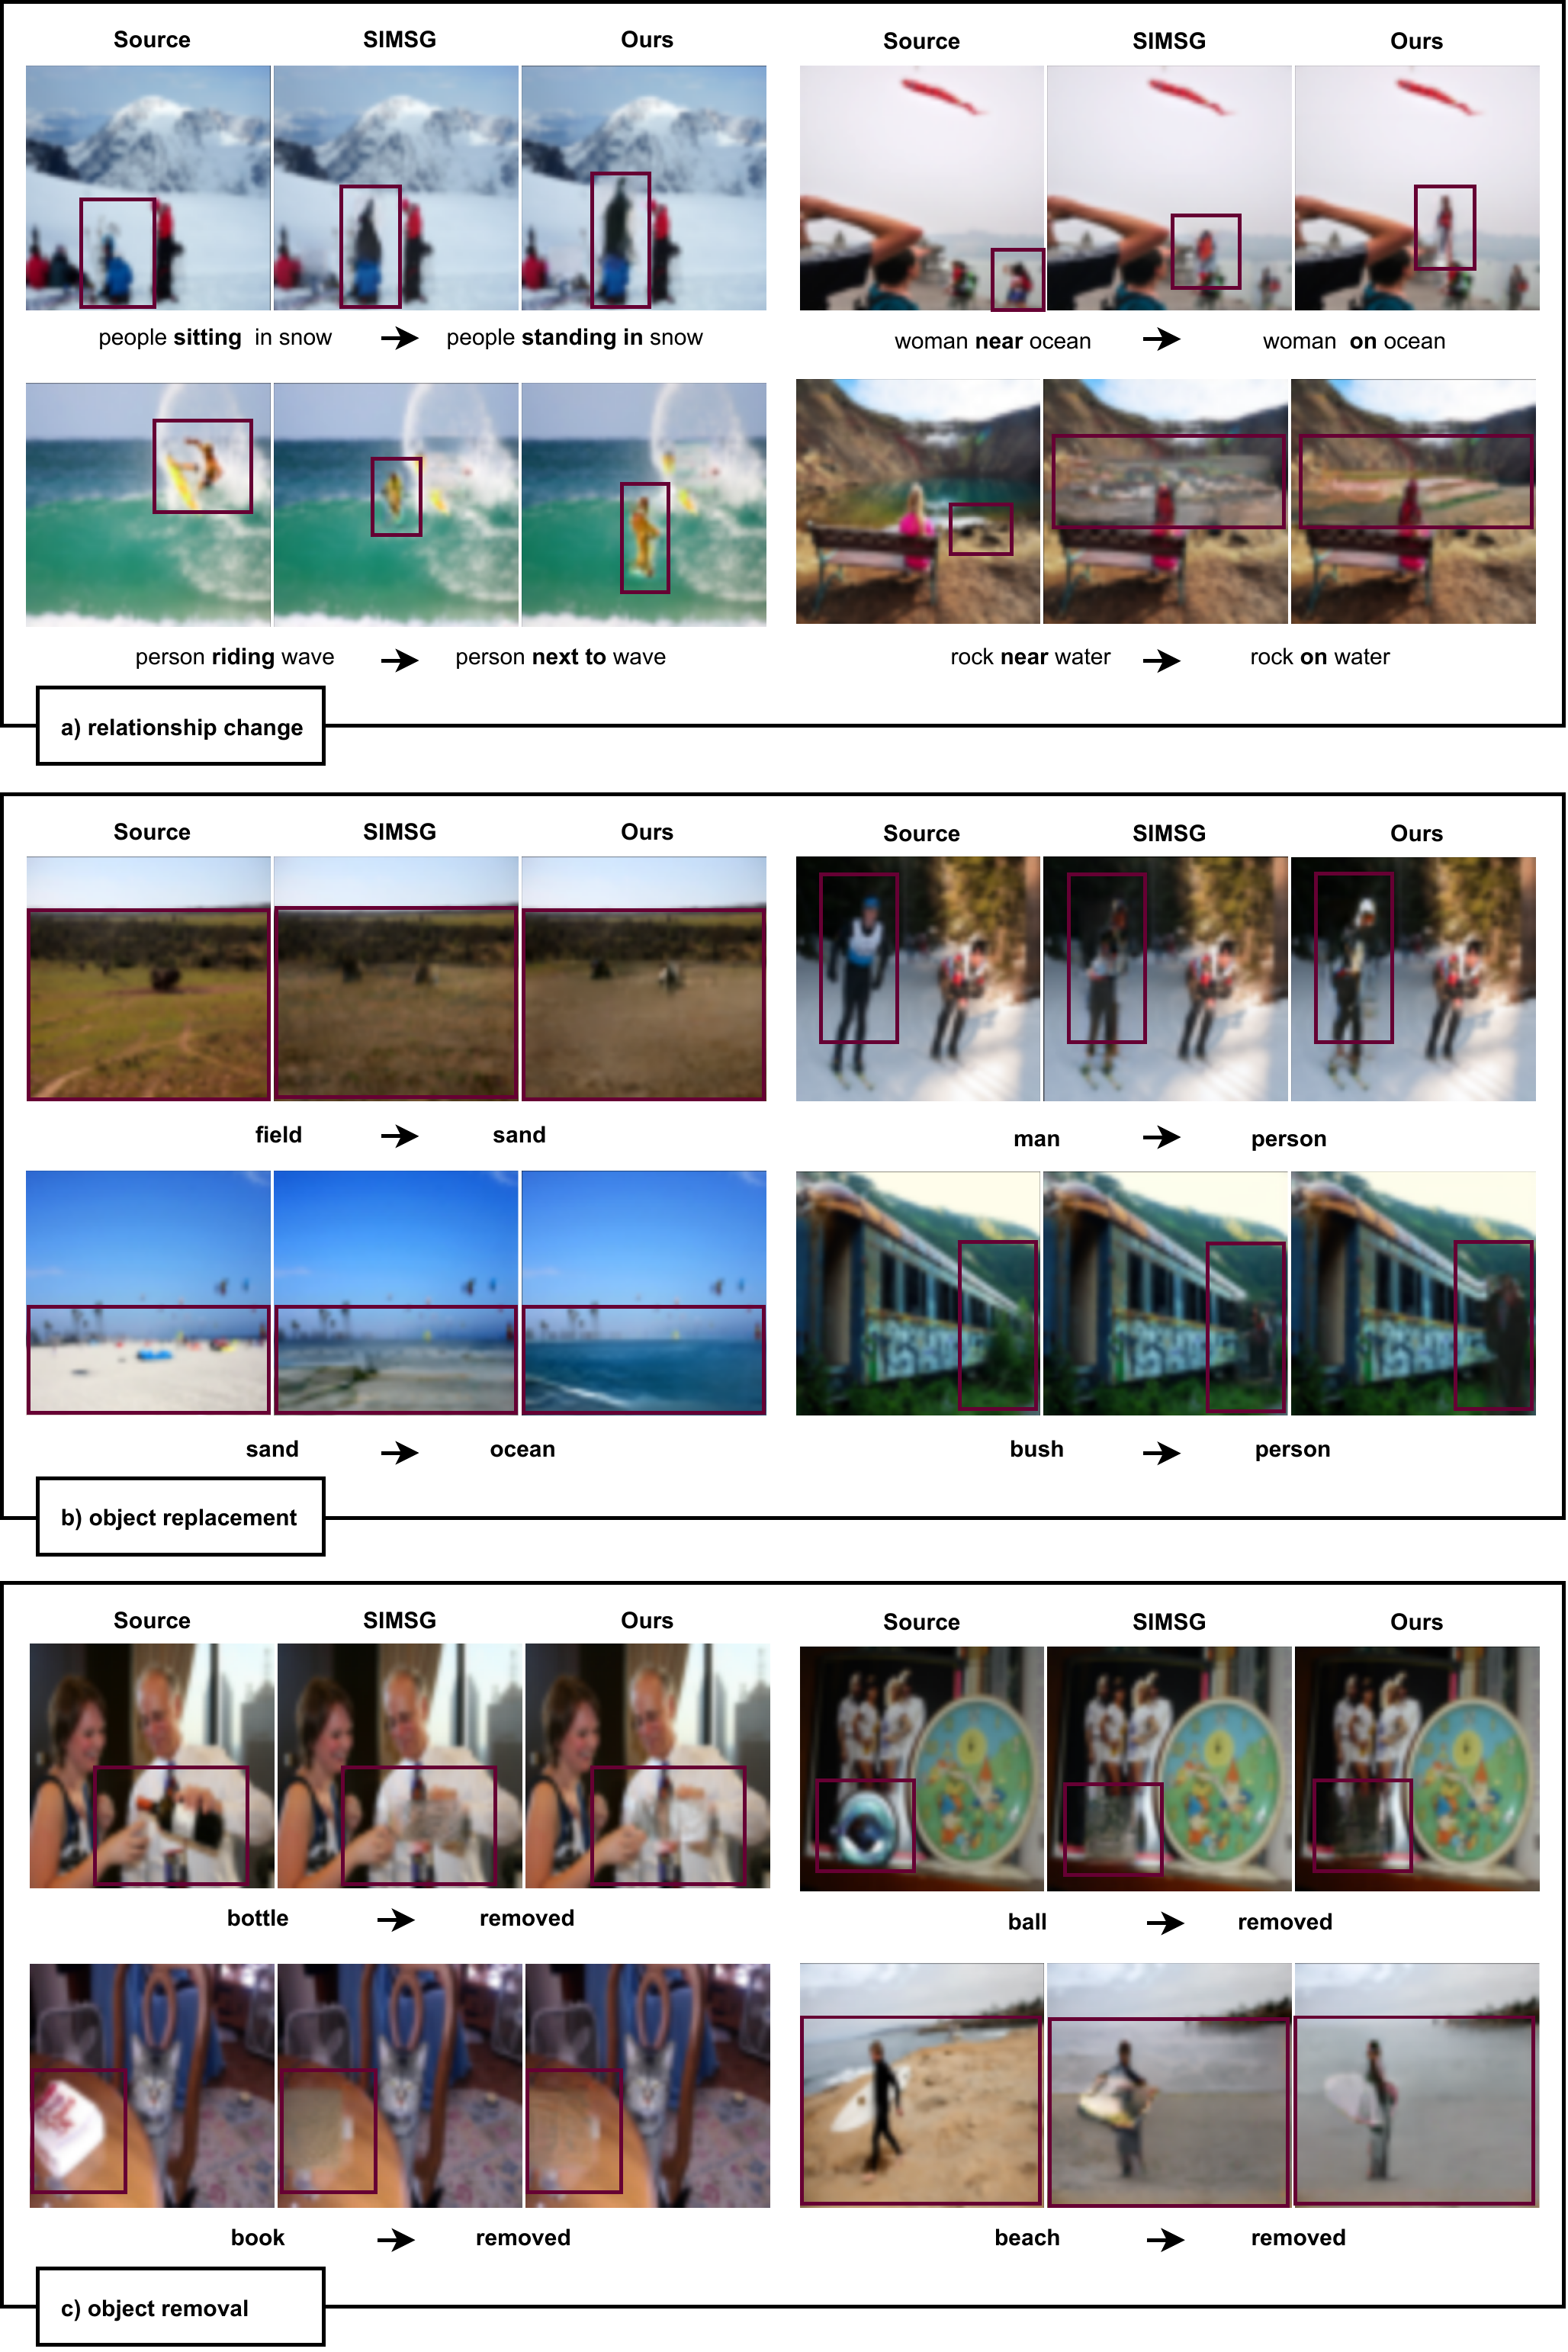}
    \caption{Additional qualitative results for image manipulation on VG}
    \label{fig:qual_res}
\end{figure}

\section{Diversity Comparison Results}
Our method is able to generate more diverse images compared to SIMSG \cite{dhamo2020semantic}. The reason behind this diversity is the variational representation for the object features, which enables probabilistic sampling of features in the latent space. However, the diversity of the generated images by our model sometimes comes with a cost of quality loss in the objects. For example, as seen in \cref{fig:diversity}, the sand generated by our model can also look like grass which is not realistic. Therefore, our model is more beneficial in scenarios where higher diversity is needed.

\begin{figure*}
    \centering
    \includegraphics[width=\textwidth]{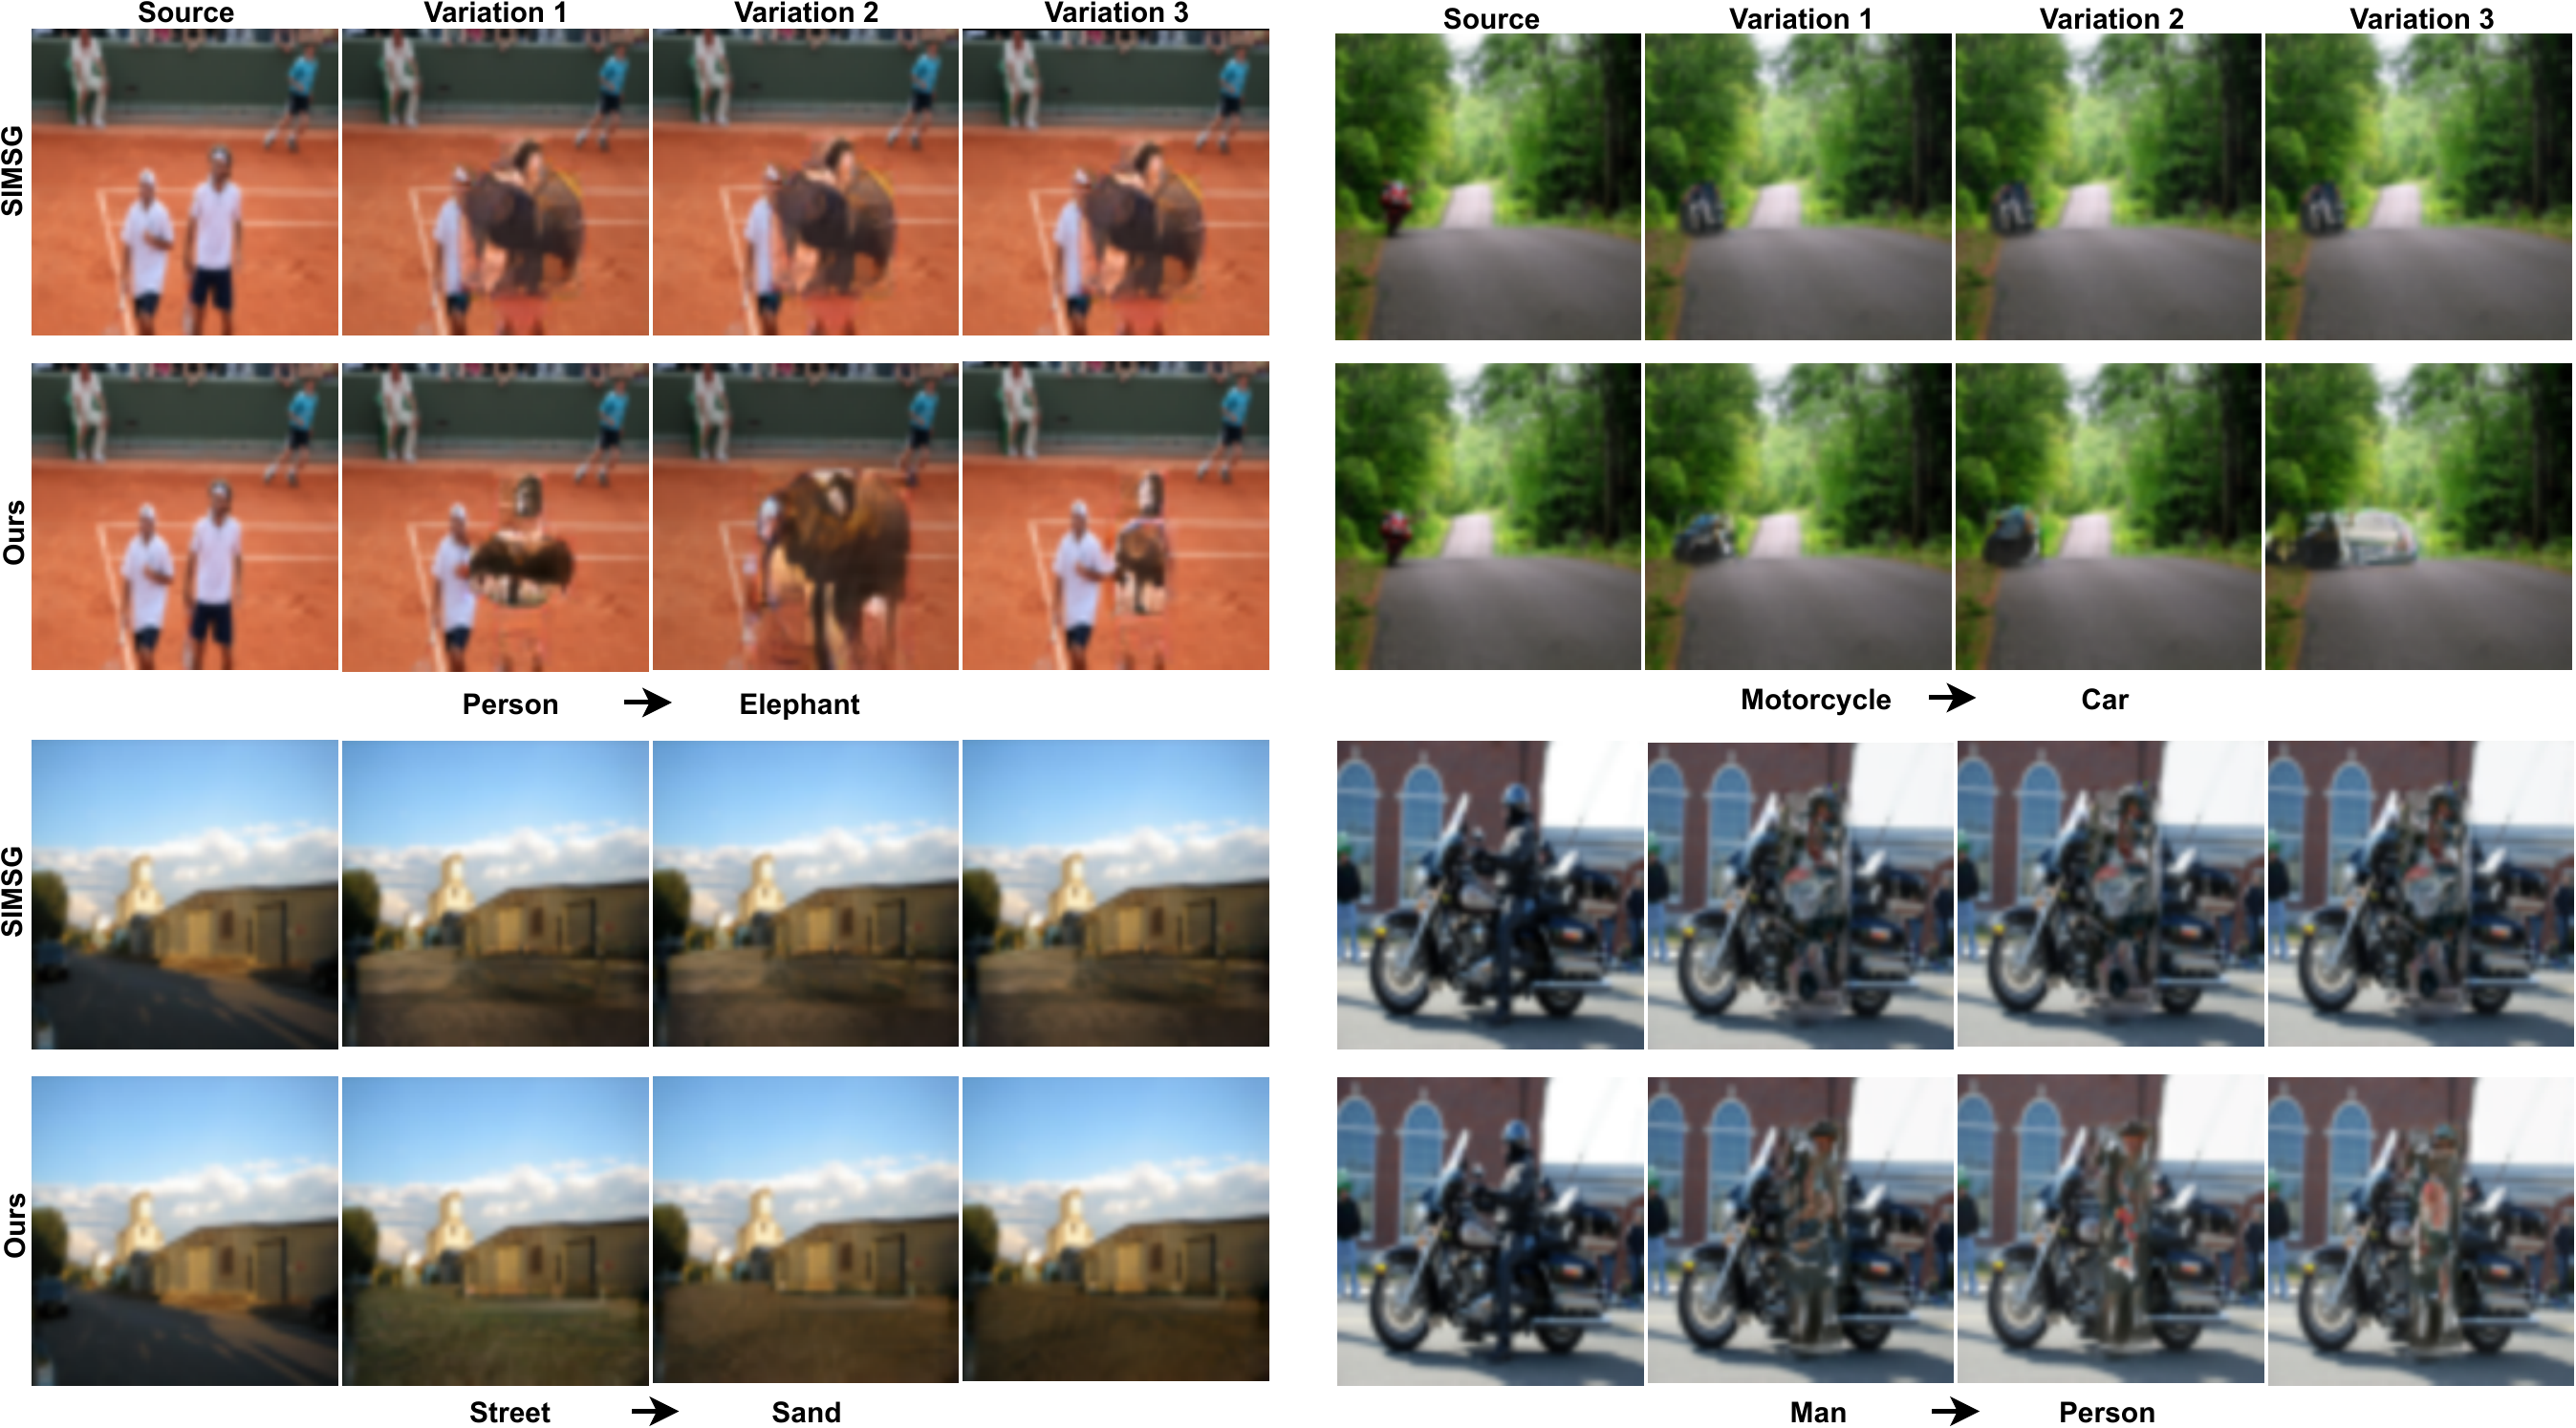}
    \caption{\textbf{Diversity in image generation.} As a result of using variational embedding in the object features, our model is able to generate diverse images in contrast to the previous work. As it can be seen, our model generated objects with different textures, sizes, and colors, while SIMSG generated the same image over different iterations.}
    \label{fig:diversity}
\end{figure*}

\section{User Study}
In order to compare the qualitative results of our method to the SIMSG baseline \cite{dhamo2020semantic}, we have performed a user study for different image manipulation modes on the Visual Genome \cite{krishna2017visual} dataset. The user study consists of 21 questions with images before and after the manipulation by the two methods. The users had to choose the image that corresponds better to the specified change. The number of participants in the user study is $37$ and the summary of their responses is provided in the main paper. The order of the methods for each example in the study is kept random, to avoid bias. The values reported in the user study table provided in the main text, shows the percentage of images chosen as having higher quality and correspondence to the specified change by the participants. The results show that our method significantly outperforms SIMSG in all manipulation modes. 

\section{Architecture Details}

\subsubsection{DSGN architecture} The input to the DSGN is the visual features from a VGG-16~\cite{simonyan2014very} network, bounding box coordinates, node embeddings, and the edge embeddings, along with the edges. The DSGN has two subnetworks, with the same architecture shown in \cref{tab:gcn_arch}. The first network produces latent features by applying the edge information to the concatenated features. The second network receives these latent features and produces the final object features, which are later used by the pose and appearance encoder network. Each DSGN subnetwork reduces the input dimensionality via a Sparse input layer \cite{feng2017sparse} to $k * nhidden$, where $nhidden=14$ is the size of the hidden dimension in the neighborhood routing (NeibRouting) layer, and $k=16$ determines the disentangling factor. The routing is performed for $12$ iterations for each of the $10$ NeibRouting layers. The output of these layers is then processed by a fully connected layer, 1D Batchnnorm, and an activation function. %, which is also the number of capsules in the NeibRouting layer

\begin{table}[]
    \centering
    \caption{DisenGCN Architecture}
    \begin{tabular}{|c|}
    \hline
         \textbf{Input}: node\_features (node\_dim), edges (edge\_dim) \\ \hline
         SparseInputLayer (node\_dim, k * nhidden) \\ \hline
         LeakyRelu \\ \hline
         10X NeibRouting (k * nhidden) \\ \hline
         FC (k * nhidden, out\_dim) \\ \hline
         BatchNorm1D (out\_dim) \\ \hline
         LeakyRelu \\ \hline
         \textbf{Output}: $z_\mathcal{G}$ (out\_dim) \\ \hline
    \end{tabular}
    
    \label{tab:gcn_arch}
\end{table}

\subsubsection{Appearance decoder $Q_A$} The appearance decoder network consists of $5$ SPADE Residual Blocks from the original implementation \cite{park2019SPADE} with up-sampling layers in between, followed by a Conv2D, an activation function, and another Conv2D layer as shown in \cref{tab:spade_arch}.

\begin{table}[]
    \centering
    \caption{Appearance decoder architecture}
    \begin{tabular}{|c|}
    \hline
         \textbf{Input}: $z_l$ (in\_dim) \\ \hline
         SPADEResBlock (in\_dim, 1024) \\ \hline
         Upsample (scale=2) \\ \hline
         SPADEResBlock (1024, 512) \\ \hline
         Upsample (scale=2) \\ \hline
         SPADEResBlock (512, 256) \\ \hline
         Upsample (scale=2) \\ \hline
         SPADEResBlock (256, 128) \\ \hline
         Upsample (scale=2) \\ \hline
         SPADEResBlock (128, 64) \\ \hline
         Conv2D (64, 64, kernel=(3,3), padding=1) \\ \hline
         LeakyRelu \\ \hline
         Conv2D (64, 3, kernel=(1,1)) \\ \hline
         \textbf{Output}: Image (64, 64, 3) \\ \hline
    \end{tabular}
    
    \label{tab:spade_arch}
\end{table}

\subsubsection{Encoder architectures}
For both $E_A$, $E_P$, we use small convolutional networks to encode the object features. Both encoders have the same architecture and consist of two encoders, one for modeling data mean $\mu$ and one for the data variance $\sigma$. The variance encoder branch has a \textit{SoftPlus} activation layer in the output. \cref{tab:encoder_arch} shows the architecture of the encoders.

\begin{table}[]
    \centering
    \caption{Encoder Architecture}
    \begin{tabular}{|c|}
    \hline
         \textbf{Input}: $z_\mathcal{G}$ (in\_dim) \\ \hline
         BatchNorm2D (in\_dim) \\ \hline
         Conv2D (in\_dim, 128, kernel=(1,1), stride=1) \\ \hline
         LeakyRelu \\ \hline
         BatchNorm2D (128) \\ \hline
         Conv2D (128, in\_dim, kernel=(1,1), stride=1) \\ \hline
         LeakyRelu \\ \hline
         \textbf{Output}: $z_{\mathcal{G}A/P}$ (in\_dim)\\ \hline
    \end{tabular}
    
    \label{tab:encoder_arch}
\end{table}

\subsubsection{Pose Decoder $Q_P$} The pose decoder network $Q_P$ receives the latent embeddings from the pose encoder $E_P$ and outputs a vector with the size of $6$ per object for each of the transformation parameters. As shown in \cref{tab:decoder_arch}, the final output has the shape of $out\_dim$, which is equal to $6$ here. Similar to the encoders, the $Q_P$ has two subnetworks with the same architecture for modeling $\mu$ and $\sigma$. The $\sigma$ branch, again has a \textit{SoftPlus} layer in the output.
        
\begin{table}[]
    \centering
    \caption{Pose Decoder Architecture}
    \begin{tabular}{|c|}
    \hline
         \textbf{Input}: $z_{\mathcal{G}P}$ (in\_dim) \\ \hline
         FC (in\_dim, 64) \\ \hline
         LeakyRelu \\ \hline
         FC (64, out\_dim) \\ \hline
         LeakyRelu \\ \hline
         \textbf{Output}: $\gamma$ (out\_dim = 6)\\ \hline
    \end{tabular}
    \label{tab:decoder_arch}
\end{table}

\subsubsection{Discriminator architecture} Both global and local discriminators follow the implementation of Multiscale Discriminator from SPADE \cite{park2019SPADE}. There are three discriminator networks at different scale values, with each having 3 Conv2D layers.

\section{Experimental Setting} The weighting hyperparameters are presented in \cref{tab:lambdas}. The optimizer used for all the experiments is Adam ~\cite{kingma2014adam} with an initial learning rate of $0.0002$. The batch size used for all trainings is set to $32$. %The models were trained on a single NVIDIA Titan V, which takes five days for 300k iterations.

\begin{table}[h]
    \centering
    \caption{Loss weighting multiplier values}
    \begin{tabular}{|l|c|}
    \hline
        Weight Multiplier & Value \\
        \hline
       $\lambda_o$ & $0.1$ \\ %
       $\lambda_a$ & $0.1$\\ %
       $\lambda_g$ & $1$ \\ %
     $\lambda_f$ & 10 \\
        $\lambda_p$ & 10 \\
        $\lambda_b$ & 50 \\
       \hline
    \end{tabular}
    \label{tab:lambdas}
\end{table}
